# Supplementary material for: Temporal Reasoning Through Automatic Translation of tock-CSP into Timed Automata
Source: arXiv:2104.13434 source file (2021-04-27)
Supplement: Supplementary file 1 [file appendixRules.tex]

\subsection{An Overview of the Translation Rules}
